# Supplementary material for: MMO: Meta Multi-Objectivization for Software Configuration Tuning
Source: arXiv:2112.07303 source file (2024-03-15)
Supplement: Supplementary file 1 [file appendix.tex]

\section{}
%\section{Proof for the MMO Model}
\label{sec:app}

\begin{remark}
	The global optimum of the original single-objective problem is Pareto optimal in MMO.
\end{remark}

\begin{proof} (By contradiction)
	Let the global optimum of the original single-objective problem be $\vect{p}$.
	Then, $\forall \vect{x} \in \mathbfcal{X}, f_t(\vect{p}) \leq f_t(\vect{x})$.
	Assuming that $\vect{p}$ is not a Pareto optimal solution for the MMO model of Equation~\ref{Eq:model}, 
	then there exists at least one solution $\vect{q}$ 
	such that $\vect{q} \prec \vect{p}$. 
	That is 
	\begin{align*}
	\begin{split}
	\begin{cases}
	f_t(\vect{q}) + w f_a(\vect{q}) < f_t(\vect{p}) + w f_a(\vect{p}) \\
	f_t(\vect{q}) - w f_a(\vect{q}) \leq f_t(\vect{p}) - w f_a(\vect{p}) \\
	\end{cases}
	\end{split}
	\end{align*}
	or 
	\begin{align*}
	\begin{split}
	\begin{cases}
	f_t(\vect{q}) + w f_a(\vect{q}) \leq f_t(\vect{p}) + w f_a(\vect{p}) \\
	f_t(\vect{q}) - w f_a(\vect{q}) < f_t(\vect{p}) - w f_a(\vect{p}) \\
	\end{cases}
	\end{split}
	\end{align*}
	
For either of the above equations, 
adding up the left and right sides of the two parts, respectively,
we have $2f_t(\vect{q}) < 2f_t(\vect{p})$, 
a contradiction to $\vect{p}$ being the global optimum of the problem. 	
\end{proof}
